# Supplementary material for: Detecting Malicious Source Code in PyPI Packages with LLMs: Does RAG Come in Handy?
Source: arXiv:2504.13769 source file (2025-04-18)
Supplement: Supplementary file 1 [file appendixs.tex]

% \documentclass{article}
% \usepackage{tabularx}
% \usepackage{geometry}
% \usepackage{hyperref}
% \usepackage{tabularx}
% \usepackage{subcaption}
% \usepackage{subfigure}

% \begin{document}

\section{Appendix }

\appendix

\subsection{A: Prompts}
\Subsubsection{RQ1: LLM Analysis Prompts}

This appendix provides the structured prompts used for zero-shot file analysis and overall package risk assessment in our study.

\subsection{Zero-Shot File Analysis Prompt}
The following prompt was used to analyse individual files within a package:

\begin{quote}
\textbf{Role: Developer}  
You are a cybersecurity expert analyzing potential malware. Read the file content in \texttt{\{file\_name\}} below and determine if it is Malicious or Benign. Explain your decision in detail.  

\textbf{Answer Format:}  
- **Predicted Classification**: (Malicious or Benign)  
- **Malicious Score**: (0-100, where 100 means highly malicious)  
- **Explanation**: (Brief description of why it is classified this way in two sentences?)  
\end{quote}

\begin{quote}
\textbf{Role: User}  
\texttt{file content: \{file\_content\}}  
\end{quote}

\subsection{Overall Package Risk Analysis Prompt}
The following prompt was used to determine the overall risk level of a package based on multiple file analyses:

\begin{quote}
\textbf{Role: User}  
Given the analysis of multiple files in a package, determine the overall risk.  

\textbf{Input Data:}  
- Number of Malicious Files: \texttt{\{malicious\_count\}}  
- Number of Benign Files: \texttt{\{benign\_count\}}  
- Average Malicious Score: \texttt{\{avg\_malicious\_score:.2f\}}  

\textbf{Answer Format:}
\begin{enumerate}
    \item **Overall Classification**: (Malicious or Benign)
    \item  **Overall Malicious Score**: (0-100, where 100 means highly malicious)  
    \item 
    **Overall Explanation**: (Brief description of why it is classified this way in two sentences?) 
    
\end{enumerate}
\end{quote}

\begin{quote}
\textbf{Role: User}  
Provide a summary explanation about whether the overall package should be classified as malicious or benign given this information:  
\texttt{\{package\_info\}}  
\end{quote}

\section{Research Question-Specific Prompts}

\subsection{RQ1: General LLM Capabilities}  
This prompt was used to evaluate whether open-source LLMs can detect malicious intent in code and packages as effectively as proprietary LLMs.

\subsection{RQ2: RAG-Enhanced LLM Capabilities}  
This prompt was used to assess the impact of Retrieval-Augmented Generation (RAG) on improving the detection of malicious intent in code.

\subsection{RQ3: Fine-Tuning Performance}  
This prompt was used to determine how well a fine-tuned open-source LLM performs in detecting malicious code.

\subsection{RQ4: Fine-Tuning and RAG Combined}  
This prompt was used to evaluate the effectiveness of combining fine-tuning with RAG for detecting malicious code.
\subsection{B: YARA RULES}

% \end{document}
